# Supplementary material for: ROAM: Reinforcement Learning Optimized Adaptive Moving Target Defense for Smart Grid
Source: arXiv:2610.12730 source file (2026-10-08)
Supplement: Supplementary file 1 [file Appendix.tex]

%   \section{Appendix A}
% \subsection{Modeling Notations}
% \label{sub:notations}


% % \begin{table}[!t]
% % % \centering
% % \caption{Modeling Notations}
% \label{tab:modeling-notations}
% %\scriptsize
% \small
% \begin{tabular}{p{2cm} p{1cm}  p{4.5cm}  }
% \hline
% \textbf{\begin{tabular}[c]{@{}l@{}}Type of\\ Notation\end{tabular}}                         & \textbf{Notation} & \textbf{Description} \\ \hline
% %%%%%%%%%%%%%%%%%%%%%%%%%%%%%%%%%
% \multirow{}{}{\textbf{General}} 
% & $\mathcal{B}$ & Set of all buses in the system \\ 
% & $\mathcal{B}^{\mathit{PV}}$ & Set of generator buses    \\        
% & $\mathcal{B}^{\mathit{GV}}$ & Set of generator buses with governors  \\
% & $\mathcal{B}^{\mathit{PQ}}$ & Set of load buses \\ 
% & $\mathcal{B}^{S}$           & Slack bus   \\   
% & $\mathcal{G}$               & Set of all generators  \\     
% & $\mathcal{T}^{P, S, T}$       & Set of all timeslots for primary, secondary, and tertiary  controllers' response  \\ 
% & $\mathcal{V}_{wac}$                  & WAMPAC signal for generator \\
% & $\mathcal{Z}$                  & Set of all areas \\
% & b, c                   & indices for  buses \\
% & i, j                   & indices for  areas \\
% \\ \hline
% %%%%%%%%%%%%%%%%%%%%%%%%%%%%%%%%%%%%%%%%%%%%%%
% \multirow{}{}{\textbf{\begin{tabular}[c]{@{}l@{}}Bus\\ Measurements\end{tabular}}}        
% & $\delta$                  & Phase angle of bus\\

% & $\mathcal{P}_{\mathit{L}}$ & Load active power  \\ 

% & $\mathcal{V}_{\mathit{t}}$ & Bus voltage  \\ 

% & $\mathcal{F}_{\mathit{t}}$ & Bus Frequency \\
% \hline
% %%%%%%%%%%%%%%%%%%%%%%%%%%%%%%%%%%%%%%%%%%%%%%
% \multirow{}{}{\textbf{\begin{tabular}[c]{@{}l@{}}Generators\\ Measurements\end{tabular}}} & 

% $\mathcal{P}_{\mathit{g}}$ & Electrical power of the generator\\ 
% & $\mathcal{P}_{\mathit{m}}$ & Mechanical power of the govornor\\
% & $\mathcal{P}_{\mathit{r}}$ & Reference set point of the generator \\          
% & $\delta$                  & Rotor angle of the generator \\
% & $\omega$              & Angular frequency of the generator \\
% & $\mathcal{V}_{ref}$  & Reference voltage of AVR in generators \\
% & $\mathcal{V}_{pss}$  & Output signal of PSS in generators \\
% & $\mathcal{V}_{avr}$  &  Output signal of the avr in generators \\
% & $\mathcal{V}_{r}$  &  Output signal of the stator in generators \\
% & $\mathcal{E}_{fd}$  &  Induced voltage of stator in generators \\
% \hline 
% %%%%%%%%%%%%%%%%%%%%%%%%%%%%%%%%%%%%%%%%%%%%%%
% \multirow{}{}{\textbf{\begin{tabular}[c]{@{}l@{}}Fixed \\ Parameters\end{tabular}}}       
% & $\mathcal{R}$                & Droop characteristics of generator \\ 
% & $\Delta T$                       & Discretized time-step size(s)  \\
% & $\mathcal{T}$                & Time-constant of the generator \\                        
% & $\mathcal{B}_{A}$   & Imaginary part of line admittance (siemens)\\
% & $\mathcal{G}_{A}$   & Real part of line admittance (mho) \\
% & $\omega_{s}$              & Reference angular frequency  \\
% & $\mathcal{\delta}_{s}$      & Reference rotor angle of the slack bus  \\
% & $\mathcal{H} $     & Inertia constant of generator\\ 
% & $\mathcal{K}_{P}$     & Proportional constant\\ 
% & $\mathcal{K}_{I}$     & Integral constant \\ 

% & $\mathcal{K}_{D}$     & Derivative constant\\ 


% \hline
% % \multirow{1}{*}{\textbf{\begin{tabular}[c]{@{}l@{}}Variable \\ Parameters\end{tabular}}}     
% % & $\mathcal{ACE}^{i}_{t}$ & Area control error of area $i$ at time $t$ (i.e., $i$ $\in$ $\mathcal{Z}$) \\

% % & $\mathcal{ACE}^{b}_{t}$ & Area control error for the generator connected to bus $b$ at time $t$ (i.e., $b$ $\in$ $\mathcal{B}^{\mathit{GV}}$) \\
% % \\ \hline

% \multirow{}{}{\textbf{\begin{tabular}[c]{@{}l@{}} BDD \\ Parameter\end{tabular}}}     
% & $\tau_{\omega} $ & BDD threshold for frequency \\

% & $\tau_{wac} $ & BDD threshold of WAMPAC signal\\
% % & $\tau_{tie}^i $ & Bad data detection threshold for tie line power of area i \\
% & $\tau_{v} $ & BDD threshold for voltage \\
% & $\epsilon_{\omega}$ & Slack term for frequency attack at AGC\\ 
% & $\epsilon_{wac}$ & Slack term for frequency attack at WAMPAC\\ 
% & $\epsilon_{v}$ & Slack term for attack on voltage at AVR \\ 
% & $\bar{\tau}_f $ & Over and under frequency threshold \\
% & $\bar{\tau}_{v}$ & Over and under voltage threshold \\ \hline

% \end{tabular}
% % \normalsize
% % \end{table}
% %%%%%%%%%%%

% \subsection{Generator and Governor Parameters}
% \label{sub:generator_parameters}
% %%%%%%%%%%%%
% \begin{table}[H]
% \centering
% \label{tab: generator_parameters}
% \begin{tabular}{|c|c|c|c|}
% \hline
% \textbf{Bus No.} & \begin{tabular}[c]{@{}c@{}}$H(s)$\end{tabular}  & \textbf{$R(p.u.)$} & \textbf{$T(s)$} \\ \hline
% 30 & 4.20 & 0.05 & 0.50 \\ \hline
% 31 & 3.03 & 0.05 & 0.50 \\ \hline
% 32 & 3.58 & 0.05 & 0.50 \\ \hline
% 33 & 2.86 & 0.05 & 0.50 \\ \hline
% 34 & 2.60 & 0.05 & 0.50 \\ \hline
% 35 & 3.48 & 0.05 & 0.50 \\ \hline
% 36 & 2.64 & -    & -    \\ \hline
% 37 & 2.43 & -    & -    \\ \hline
% 38 & 3.45 & -    & -    \\ \hline
% 39 & 50.00 & 0.05   & 0.05    \\ \hline
% \end{tabular}
% \vspace{-10pt}
% \end{table}
% %%%%%%%%%%%%%%%%%%%%

% \subsection{Simulation and Modeling Parameters}
% \label{sub:simulation_parameters}
% %%%%%%%%%%%%%%%%%%%%
% \begin{table}[H]
% \centering
% \label{tab:simulation_parameter}
% \begin{tabular}{|c|c|c|c|}
% \hline
% \textbf{Parameter} & \textbf{Value} & \textbf{Parameter} & \textbf{Value} \\ \hline
% $\mathcal{F}_s$ (Hz)         & 60.00          & $\overline{\tau_{\omega}}$ (p.u.) & 1.008 \\ \hline
% $\Delta T$ (s)            & 1/60           & $\overline{P}_{m,max}^b$ (p.u.)    & 1.10 \\ \hline
% $S^b$ (MVA) & 1.00           &      $ACE^b$ (p.u.)               & $\pm$0.05 \\ \hline
% $\overline{\tau_{v}}$ (p.u.)    & 1.10           & $\overline{\tau_{wac}}$ (p.u.) & 1.008 \\ \hline
% $\mathcal{K}^{b}_{P-wac}$   & 0.01     & $\mathcal{K}^{b}_{P-avr}$      & 0.75 \\ \hline
% $\mathcal{K}^{b}_{I-wac}$   & 0.01     & $\mathcal{K}^{b}_{I-avr}$       & 1 \\ \hline
% $\mathcal{K}^{b}_{D-wac}$   & 0.01     & $\mathcal{K}^{b}_{D-avr}$   & 0.25 \\ \hline
% \end{tabular}
% \end{table}
% %%%%%%%%%%%%%%%%%%%%





% \subsection{Linearization Process}
% \label{sub: linearized_model}
% %
% The Backward Euler method is a numerical technique for discretizing dynamic non-linear equations, especially for stiff systems. The general form of the Backward Euler method for a first-order ordinary differential equation \( \frac{dy}{dt} = f(y, t) \) is given by:
% %%%%%%%%%%%%%%%%
% \begin{equation}
% y_{n+1} = y_n + \Delta t \cdot f(y_{n+1}, t_{n+1})
% \end{equation}
% Here, \( y_{n+1} \) is the value of the function at the next time step, \( y_n \) is the value at the current time step, and \( \Delta t \) is the time step size. Since the function \( f \) is evaluated at the future time step \( t_{n+1} \), the method is implicit, requiring the solution of an algebraic equation at each time step. 


% % The Backward Euler method is a well-known numerical technique used to discretize differential equations, particularly useful for stiff systems where stability is a concern. This implicit method approximates the derivative of a function at a future time step, providing improved stability over explicit methods like the Forward Euler method. The general form of the Backward Euler method for a first-order ordinary differential equation \( \frac{dy}{dt} = f(y, t) \) is given by:
% % %%%%%%%%%%%%%%%%
% % \begin{equation}
% % y_{n+1} = y_n + \Delta t \cdot f(y_{n+1}, t_{n+1})
% % \end{equation}
% % Here, \( y_{n+1} \) is the value of the function at the next time step, \( y_n \) is the value at the current time step, and \( \Delta t \) is the time step size. Since the function \( f \) is evaluated at the future time step \( t_{n+1} \), the method is implicit, requiring the solution of an algebraic equation at each time step. The Backward Euler method is advantageous for linearizing and solving the differential equations governing system behavior in power system dynamics. By applying this method, we transform continuous-time system dynamics into a discrete-time format that facilitates the analysis and optimization of control strategies.

% % For instance, when linearizing the system dynamics for WAMPAC under FDI attacks, the Backward Euler method discretizes equations that describe the interaction between PSS, AVR, and other control elements. This results in a set of discrete-time equations that can be analyzed to determine the optimal attack vectors and assess the impact of FDI on system stability. To find out the optimal attack vectors for FDI attack in WAMPAC we have linearized the above system dynamics using Backward Euler's method that are presented in Eqn.~\ref{eq:pss-equation}-~\ref{eq:delta_new}:
% %%%%%%%%%%%%%%%%
% \begin{equation}
%     \label{eq:pss-equation}
%     \begin{split}
%      \mathcal{V}_\mathit{pss, t+1}^{b} = \mathcal{K}_\mathit{pss}^{b} (\omega_{t+1}^b - \omega_{s}) 
%      % +\mathcal{K}^\mathit{wac}_{b}*(\sum_{i,j=1}^{3, i \neq j}\Delta \omega^\mathit{area}_{i}-\Delta \omega^\mathit{area}_{j})  
%      \end{split}
% \end{equation}
% \begin{equation}
%     \begin{split}
%        &\mathcal{V}_{wac, t+1}^{b} =\mathcal{V}_{wac, t}^{b}+ \mathcal{K}_{p-wac}^b* \Delta \omega_{Area,t+1}^{ij}+\mathcal{K}_{i-wac}^b \\& *  \Delta \omega_{Area,t+1}^{ij}* \Delta T +  \mathcal{K}_{d-wac}^b*\frac{\Delta \omega_{Area,t+1}^{ij}-\Delta \omega_{Area,t}^{ij}}{\Delta T}
%     \end{split}
% \end{equation}
% \begin{equation}
%  \mathcal{V}_{pss-total, t+1}^b = \mathcal{V}_{pss, t+1}^b +  \mathcal{V}_{wac,t+1}^{b} 
% \end{equation}

% % \begin{equation}
% %     \label{eq:pss-equation}
% %     \begin{split}
% %      \mathcal{V}^\mathit{wac}_{b, t+1} =
% %      \mathcal{K}^\mathit{pss}_{b} (\omega_{b,t} - \omega_{s})+\mathcal{K}^\mathit{wac}_{b}*(\sum_{i,j=1}^{3, i \neq j}\Delta \omega^\mathit{area}_{i}-\Delta \omega^\mathit{area}_{j})
% %     \end{split}
% % \end{equation}
% % \begin{equation}
% %     \label{eq:vref-equation}
% %     \begin{split}
% %      \mathcal{V}^\mathit{ref}_{b, t+1} = \mathcal{V}^\mathit{steady}_{b} *\{1+ \mathcal{K}^\mathit{exc}(\omega_{b, \mathit{t}} - \omega_{s})\}
% %     \end{split}
% % \end{equation}
% \begin{equation}
%     \label{eq:ve-equation}
%      \mathcal{V}_\mathit{e,t+1}^{b} = \mathcal{V}_\mathit{ref,t+1}^{b}- \mathcal{V}_\mathit{t, t+1}^{b}- \mathcal{V}_\mathit{pss-total,t+1}^{b}
% \end{equation}
% \begin{equation}
%     \begin{split}
%        &\mathcal{V}_{avr, t+1}^{b} = \mathcal{V}_{avr, t}^{b} + \mathcal{K}_{p-avr}^b* \mathcal{V}_\mathit{e,t+1}^{b}+\mathcal{K}_{i-avr}^b* \mathcal{V}_\mathit{e,t+1}^{b} \\& * \Delta T + \mathcal{K}_{d-avr}^b*\frac{\mathcal{V}_\mathit{e,t+1}^{b}-\mathcal{V}_\mathit{e,t}^{b}}{\Delta T}
%     \end{split}
% \end{equation}
% \begin{equation}
%     \label{eq:V_e-equation}
%     \begin{split}
%      \mathcal{E}_\mathit{fd, t+1}^{b} = \mathcal{V}_\mathit{avr,t+1}^{b}- \mathcal{K}_\mathit{4}^{b} (\delta_{t+1}^b - \delta_{t}^b)
%     \end{split}
% \end{equation}
% \begin{equation}
%     \label{eq:V_ter-equation}
%     \begin{split}
%      \mathcal{V}_\mathit{t,t+1}^{b} = \mathcal{K}_\mathit{5}^{b}*(\delta_{t+1}^b -
%      \delta_{t}^b)+\mathcal{K}_\mathit{6}^{b}*(\mathcal{E}_{fd,t+1}^b -\mathcal{E}_{fd,t}^b)  
%     \end{split}
% \end{equation}
% % \begin{equation}
% %     \label{eq:activepower-equation}
% %     \begin{split}
% %      \mathcal{P}^\mathit{g}_{b,t+1} = \mathcal{P}^\mathit{g}_{b, t}+ \mathit{\Delta T}*\{\mathcal{P}^\mathit{s}_{b}*(\delta_{b,t} -
% %      \delta_{s})+\mathcal{K}^\mathit{7}_{b}*(\mathcal{E}_{b,t+1} -\mathcal{E}_{b,t})\}  
% %     \end{split}
% % \end{equation}
% % \begin{equation}
% %     \label{eq:tieline-equation}
% %     \begin{split}
% %      \mathcal{P}^\mathit{tie}_{b,t+1} =\mathcal{P}^\mathit{tie}_{b,t}+\{ \mathcal{P}^\mathit{s}_{b}*(\sum_{i,j=1}^{3, i \neq j}\Delta \delta^\mathit{area}_{i}-\Delta \delta^\mathit{area}_{j})\}
% %     \end{split}
% % \end{equation}
% \begin{equation}
%     \label{eq:tieline-equation}
%     \begin{split}
%     \Delta \mathcal{P}_{tie,t+1}^{ij} &= \mathcal{P}_s*(\Delta \delta_{Area_i,t+1}- \Delta \delta_{Area_j,t+1}) \\& + \mathcal{P}_s*(\Delta \mathcal{V}_{t-Area_i,t+1}- \Delta \mathcal{V}_{t-Area_j,t+1})
%     \end{split}
% \end{equation}
% %
% \begin{equation}
%     \label{eq:ACE-equation}
%     \begin{split}
%      \mathcal{ACE}_{t+1}^i &= (\frac{1}{\mathcal{R}^b}+\mathcal{D}^b)* (\omega_{t+1}^b - \omega_{s}^b)+ \sum_{i,j=1}^{3, i \neq j} (\mathcal{P}_\mathit{tie,t+1}^{i} \\& -\mathcal{P}_\mathit{tie,t+1}^{j})
%     \end{split}
% \end{equation}
% \begin{equation}
%     \label{eq:ref_set_point-equation}
%     \begin{split}
%      \mathcal{P}_\mathit{ref, t+1}^{b} = \mathcal{P}_\mathit{ref,t}^{b}+\mathcal{P}_\mathit{g,t+1}^{b} - \mathcal{D}^b*\mathit{\Delta T}*\mathcal{ACE}_{t+1}^i
%     \end{split}
% \end{equation}
% \begin{equation}
%     \label{eq:activepower-equation}
%     \begin{split}
%      \mathcal{P}_\mathit{m,t+1}^{b} &= \mathcal{P}_\mathit{m,t}^{b}+ \frac{\mathit{\Delta T}}{\mathcal{T}^b} *(\mathcal{P}_\mathit{ref,t+1}^{b}-(\omega_{t+1}^b - \omega_{s}^b))  * \frac{1}{\mathcal{R}^b} \\&-\mathcal{P}_\mathit{m,t+1}^{b}\
%     \end{split}
% \end{equation}
% \begin{equation}
%     \label{eq:omega}
%     \begin{split}
%      \omega_{t+1}^b = \omega_{t}^b+\frac{\Delta \delta}{2*\mathcal{H}_b}*(\mathcal{P}_{m,t+1}^{b}-\mathcal{P}_{g,t+1}^{b})
%     \end{split}
% \end{equation}
% \begin{equation}
%     \label{eq:delta_new}
%     \begin{split}
%      \delta_{t+1}^b = \delta_{t}^b+\frac{1}{\mathit{\Delta T}}*(\omega_{t+1}^b - \omega_{s}^b)
%     \end{split}
% \end{equation}
% The traditional DC model simplifies the full AC model significantly, which has led to extensive literature on optimal power flow using the DC model (e.g.,~\cite{Alguacil03TPS, Zhang12TPS}). However, the DC model assumes $\mathcal{V}_t = 1$ and cannot capture voltage dynamics, making it unsuitable for analyzing our proposed WAMPAC module, which integrates voltage and frequency dynamics of an intelligent power grid. To analyze our model, we explored the linear power flow model from~\cite{Akbari16IGT, Yang19TPS} but found the model by Vittal et al. in~\cite{Vittal13TPS} more promising. This model retains a linear representation of reactive power, off-nominal bus voltage magnitudes, and network losses. The linearization of the line flow equations is based on a Taylor series, with assumptions from ~\cite{Vittal13TPS}.

% % The approximations made in the traditional DC model significantly simplify the full AC model. As a result, much literature has been developed on optimal power flow design using the DC power flow model over the decades, i.e., \cite{Alguacil03TPS, Zhang12TPS}. However, the DC model cannot capture the voltage dynamics of the power system due to its assumption of $\mathcal{V}_t = 1$. As a result, DC power flow is unsuitable for the formal analysis of our proposed WAMPAC module, which combines an intelligent power grid's voltage and frequency dynamics.  To analyze our model, we've explored the linear power flow model mentioned in \cite{Akbari16IGT, Yang19TPS} but found the model presented by Vittal at. el in \cite{Vittal13TPS}, which retains a linear representation of reactive power, off-nominal bus voltage magnitudes, and network losses more promising. The linearization of the line flow equations is essentially based on a Taylor series, and the following assumptions are assumed to be valid as mentioned in \cite{Vittal13TPS}.

% \noindent\textit{Assumption 1:} The bus oltage magnitudes are always close to 1.0 per unit
% (p.u.).

% \noindent\textit{Assumption 2:} The angle difference across a line is small so that $\sin(\delta^b) \approx \delta^b \ $ and $\cos(\delta^b) \approx 1$ can be applied. This assumption is
% valid at the transmission level where the active power flow
% dominates the apparent power flow in the lines-
% %
% \begin{equation}
%      \mathcal{P}_{g,t+1}^b = \sum_{c=1}^{c=N} (\Delta \mathcal{V}_{t,t+1}^{b}- \Delta \mathcal{V}_{t,t+1}^{c} )\mathit{G}^{bc}_{A} \delta_{t+1}^{bc}-  \mathit{B}^{bc}_{A}\delta_{t+1}^{bc})\}
% \end{equation}
% %
% \begin{equation}
%     \begin{split}
%     \mathcal{Q}_{g,t+1}^b &= \sum_{c=1}^{c=N} -(1+ 2\Delta\mathcal{V}_{t,t+1}) \mathit{B}_{A,0}^{bc} - (\Delta \mathcal{V}_{t,t+1}^{b} \\& - \Delta \mathcal{V}_{t,t+1}^{c} )  \mathit{b}^{bc} - \mathit{G}_{A}^{bc}\delta_{t+1}^{bc})  
%     \end{split}
% \end{equation}

% % Where,$\forall_{b, c\in\mathcal{B}} $.

% \subsection{BDD Constraints of WAMPAC}
% \label{sub: BDD}
% We have formulated our optimization problem as MLIP and this type of model would not scale up for the larger system~\cite{jafari23tifs}, which is why we have combined the constraints through slack variables $\epsilon_{\omega}, \epsilon_{v}, \epsilon_{wac}$ that avoid the use of integer variables. In addition to the discretized model of WAMPAC, the below BDD constraints are used to find the optimal attack vector. The maximum and minimum values of the system parameters (i.e., the measurement of power, voltage, tangle line) are maintained according to the guideline mentioned in~\cite{NERC2016}.
% \begin{equation}
% \label{eq_bdd_1}
%     \epsilon^b_{\omega}[t] \geq 0,  \forall i \in \mathcal{B}, \forall t \in \mathcal{T}, 
% \end{equation}
% \begin{equation}
% \epsilon^b_{v}[t] \geq 0, \quad \forall i \in \mathcal{Z}, \forall t \in \mathcal{T}
% \end{equation}
% \begin{equation}
% \epsilon^b_{wac}[t] \geq 0, \forall i \in \mathcal{G}, \forall t \in \mathcal{T}
% \end{equation}
% \begin{equation}
% \omega^b[t] + \epsilon^b_{\omega}[t] \geq \bar{\tau}_{\omega}^b, \quad \forall b \in \mathcal{B}, \forall t \in \mathcal{T}
% \end{equation}
% \begin{equation}
% \mathcal{V}^b[t] + \epsilon^b_{v}[t] \geq \bar{\tau}_v^b, \quad \forall b \in \mathcal{B}, \forall t \in \mathcal{T}
% \end{equation}
% \begin{equation}
% \epsilon^b_{\omega}[t] \geq \bar{\omega}^b[t] - \bar{\omega}_b[t + 1], \quad \forall b \in \mathcal{B}, \forall t \in \mathcal{T}
% \end{equation}
% \begin{equation}
% \epsilon^b_{\omega}[t] \geq \bar{\omega}^b[t + 1] - \bar{\omega}^b[t], \quad \forall b \in \mathcal{B}, \forall t \in \mathcal{T}
% \end{equation}
% \begin{equation}
% \epsilon^b_{v}[t] \geq \bar{\mathcal{V}}^b[t] - \bar{\mathcal{V}}^b[t + 1], \quad \forall b \in \mathcal{B}, \forall t \in \mathcal{T}
% \end{equation}
% \begin{equation}
% \epsilon^b_{v}[t] \geq \bar{\mathcal{V}}^b[t+1] - \bar{\mathcal{V}}^b[t], \quad \forall b \in \mathcal{B}, \forall t \in \mathcal{T}
% \end{equation}
% \begin{equation}
% \epsilon^b_{wac}[t] \geq \bar{\mathcal{V}_{wac}}^b[t] - \bar{\mathcal{V}_{wac}}^b[t + 1], \quad \forall b \in \mathcal{B}^{PV}, \forall t \in \mathcal{T}
% \end{equation}
% \begin{equation}
% \epsilon^b_{wac}[t] \geq \bar{\mathcal{V}_{wac}}^b[t+1] - \bar{\mathcal{V}_{wac}}^b[t], \quad \forall b \in \mathcal{B}^{PV}, \forall t \in \mathcal{T}
% \end{equation}
% \begin{equation}
% P^b_{m,min} \leq P^b_{m}[t] \leq \bar{P}^b_{m,max}, \quad \forall b \in \mathcal{B}^{GV}, \forall t \in \mathcal{T}
% \end{equation}
% \begin{equation}
% P^b_{g,min} \leq P^b_{g}[t] \leq \bar{P}^b_{g,max}, \quad \forall b \in \mathcal{B}^{GV}, \forall t \in \mathcal{T}
% \end{equation}
% \begin{equation}
% Q^b_{g,min} \leq Q^b_{g}[t] \leq \bar{Q}^b_{g,max}, \quad \forall b \in \mathcal{B}^{GV}, \forall t \in \mathcal{T}
% \end{equation}
% \begin{equation}
% V^b_{t,min} \leq V^b_{t}[t] \leq \bar{V}^b_{t,max}, \quad \forall b \in \mathcal{B}^{PV}, \forall t \in \mathcal{T}
% \end{equation}
% \begin{equation}
% ACE^i_{min} \leq ACE^i[t] \leq \bar{ACE}^i_{max}, \quad \forall i \in \mathcal{Z}, 
%     \forall t \in \mathcal{T}
% \end{equation}




% % \begin{equation}
% % -\tau_{wac}^b \leq \mathcal{V}_{wac}^b[t + 1] - \mathcal{V}_{wac}^b[t] \leq \tau_{wac}^b, \quad \forall b \in \mathcal{B}^{PV},
% %     \forall t \in \mathcal{T}
% % \end{equation}
% % \begin{equation}
% %     \begin{split}
% %       -\tau_{\omega}^b \leq (\omega^b[t + 1] + \tilde{\omega}^b[t + 1]) - (\omega^b[t] + \tilde{\omega}^b[t]) \leq \tau_{\omega}^b, \\  \forall b \in \mathcal{B}^{GV}, \forall t \in \mathcal{T}  
% %     \end{split}
% % \end{equation}
% % \begin{equation}
% % \label{eq_bdd_17}
% %     \begin{split}
% %       -\tau_{V} \leq (\mathcal{V}^b_t[t + 1] + & \tilde{\mathcal{V}}^b_t[t + 1]) - (\mathcal{V}^b_t[t] + \tilde{\mathcal{V}}^b_t[t]) \\ & \leq \tau_{V}, \forall b \in \mathcal{B}^{PV}, \forall t \in \mathcal{T}  
% %     \end{split}
% % \end{equation}
% % \begin{equation}
% % \epsilon^i_{tie}[t] \geq \Delta \tilde{P}^i_{tie}[t + 1] - \Delta \tilde{P}^i_{tie}[t], \quad \forall i \in \mathcal{Z}, \forall t \in \mathcal{T}
% % \end{equation}
% % \begin{equation}
% % \epsilon^i_{tie}[t] \geq \Delta \tilde{P}^i_{tie}[t] - \Delta \tilde{P}^i_{tie}[t + 1], \quad \forall i \in \mathcal{Z},
% %     \forall t \in \mathcal{T}
% % \end{equation}
% % \begin{equation}
% % \label{eq_bdd_17}
% %     \begin{split}
% %     -\tau_{tie} \leq (\Delta P^i_{tie}[t + 1] + \Delta \tilde{P}^b_{tie}[t + 1]) - \\ (\Delta P^b_{tie}[t] + \Delta \tilde{P}_b^{tie}[t]) \leq \tau_{tie},  \forall b \in \mathcal{Z}, \forall t \in \mathcal{T}
% %     \end{split}
% % \end{equation}
